# Supplementary material for: A Machine Learning Approach for Rate Constants III: Application to the Cl($^2$P) + CH$_4$ $\rightarrow$ CH$_3$ + HCl Reaction
Source: arXiv:2206.12443 source file (2022-06-24)
Supplement: Supplementary file 1 [file SI.pdf]

# Supplementary Material: A Machine Learning Approach for Rate Constants III: Application to the Cl($^2$P)+$CH_4$→$CH_3$+HCl Reaction

Paul L. Houston,[*,†] Apurba Nandi,[‡] and Joel M. Bowman[*,‡]

†*Department of Chemistry and Chemical Biology, Cornell University, Ithaca, New York 14853, U.S.A. and Department of Chemistry and Biochemistry, Georgia Institute of Technology, Atlanta, Georgia 30332, U.S.A*

‡*Cherry L. Emerson Center for Scientific Computation and Department of Chemistry, Emory University, Atlanta, Georgia 30322, USA*

E-mail: plh2@cornell.edu; jmbowma@emory.edu

# Contents

## S-I. Experimental Data

The available experimental data are shown in Figure S1. For use in other figures in the main text, the green line in the figure shows a fit to the data of a third-order polynomial. Experimental data are identified by the first author: Clyne,[1] Manning,[2] Michael,[3] Whytock,[4] Keyser,[5] Zahniser,,[6]Ravishankara,[7] Heneghan,[8] Seeley,[9] Pilgrim,[10] and Bryukov.[11]

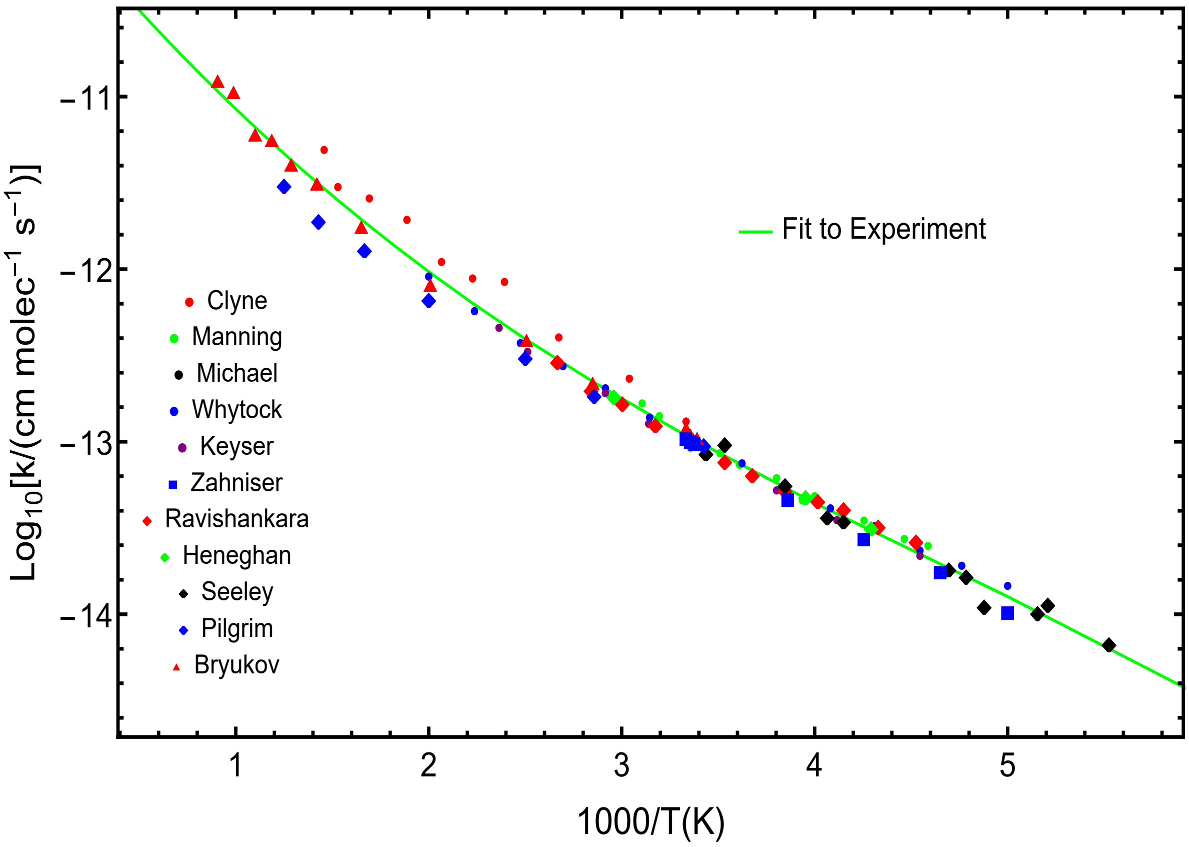


Figure S1: A fit of $\text{Log}_{10}(k)$ vs $1000/T$ for the experimental data to a $3^{rd}$-order polynomial. The fit is used to represent the experiment in some plots of the main text.

# S-II. Computational Details

Figure. S2 shows values of $\chi$ as a function of u$^*$ for the entire data set, which is largely based on a compilation by Allison and Truhlar.[12] Several features are important to note in this plot, where values of $\chi$ larger than 3.0 are shown in blue, while values lower than 3.0 are shown in red. There is a region of overlap between the two clusters for $u^*$ in the range of approximately 6 to 13. Values of $u^*$ below 5 appear only in the small-$\chi$ cluster and values of $u^*$ above 13 appear only in large-$\chi$ cluster. The question we now address is which cluster of $\chi$ should we use at a given value of u$^*$. In previous work[13] we adopted the simple expedient of using the small-$\chi$ values for temperatures corresponding to u$^*$ below 13, where the $\chi$ values were either solely in the small-$\chi$ group or where the two groups overlapped, and the large-$\chi$ values for temperatures corresponding to u$^*$ above 13, where the $\chi$ values were solely from the large-$\chi$ group. Here we use a somewhat more nuanced approach.

It is clear from Fig. S2 that we should use almost exclusively the large-$\chi$ values above u$^*$=13 and the almost exclusively the small-$\chi$ values below u$^*$=5. What we seek is a method for evaluating $\chi$ more equitably, especially in the overlap region. We approach this by noting that we can assign a raw probability (or equivalently a weight) for using the low-$\chi$ value as being the fraction of low-$\chi$ values that are above of the desired u$^*$. Similarly, a raw probability for using the high-$\chi$ value can be assigned to the fraction of high-$\chi$ values that are below the desired u$^*$. Let these raw probabilities be $P_{high}(u^*)$ and $P_{low}(u^*)$. Each is normalized within its own group, but the two probabilities are not yet normalized to one another. The correct normalization is such that $P_{high}^{norm}(u^*) + P_{low}^{norm}(u^*) = 1$, and we achieve this with the equations

$$P_{high}^{norm}(u^*) = \frac{P_{high}(u^*)}{P_{high}(u^*) + P_{low}(u^*)} \tag{S1}$$

$$P_{low}^{norm}(u^*) = \frac{P_{low}(u^*)}{P_{high}(u^*) + P_{low}(u^*)} \tag{S2}$$

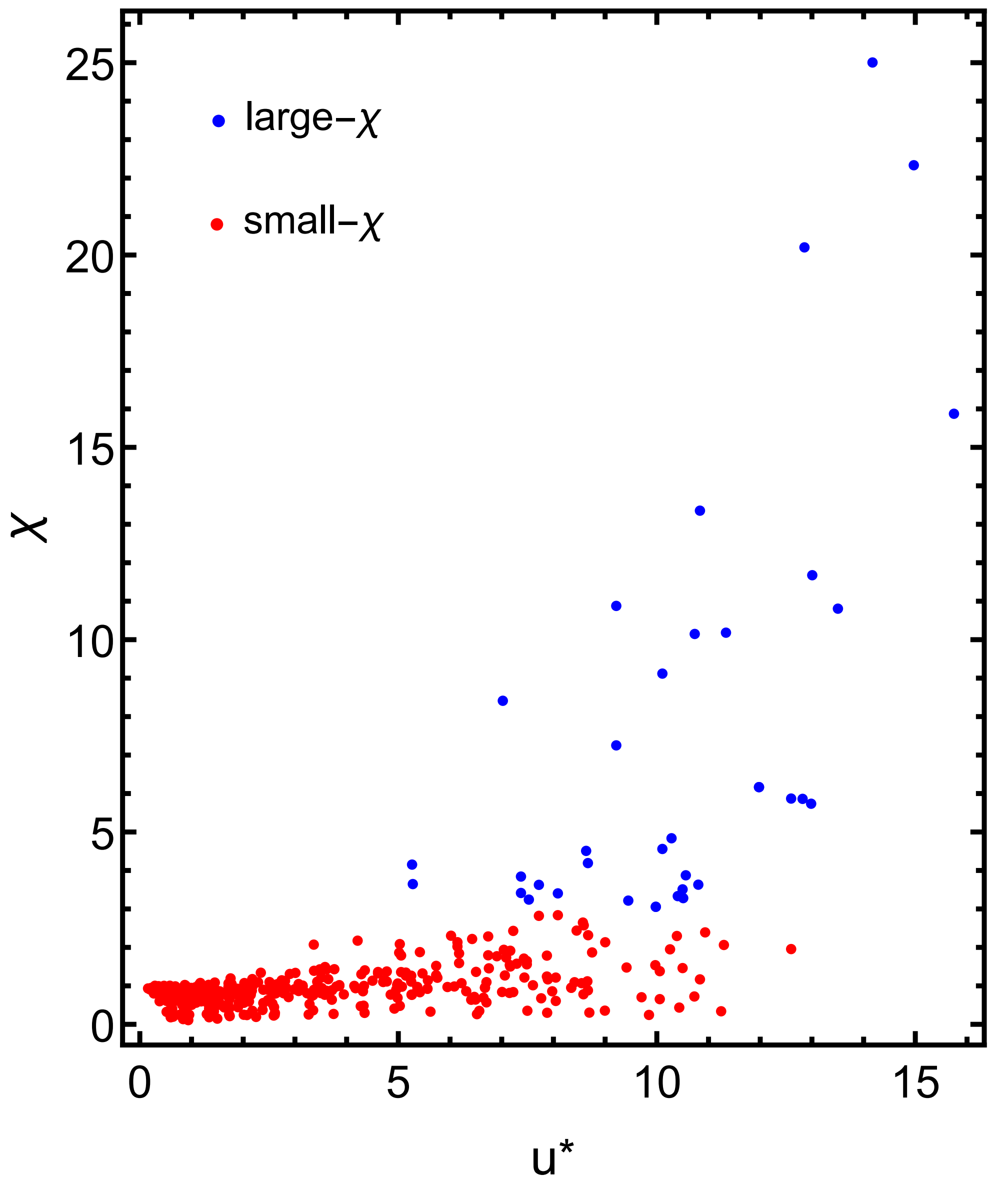


Figure S2: $\chi$ as a function of u* the entire dataset. Values above $\chi = 3.0$ are shown in blue; those below 3.0 are shown in red.

In practice, we calculate $P_{high}(u^*)$ and $P_{low}(u^*)$ from the positions of the points in Figure. S2, simply by automatic counting, and then fit the counts in each case by a suitable function that can then be used in Eqs. (S1) and (S2).

Figure S3 shows the values of $P^{norm}_{high}(u^*)$ in blue and $P^{norm}_{low}(u^*)$ in red. As expected, $P^{norm}_{high}(u^*)$ is approaches unity above u*=13, whereas $P^{norm}_{low}(u^*)$ is approaches unity below u*=5. The probabilities are equal at approximately u*=7.5, or a temperature (for the Cl

+ $CH_4$ reaction) of approximately 200 K. Thus, only the very lowest temperatures have substantial contribution from $P_{high}^{norm}(u^*)$. To find the value of $\chi$ for any value of u*, we use the formula

$$\chi(u^*) = P_{high}^{norm}(u^*)\chi_{high}(u^*) + P_{low}^{norm}(u^*)\chi_{low}(u^*) \tag{S3}$$

where $\chi_{high}(u^*)$ and $\chi_{low}(u^*)$ are the values calculated using the Gaussian Process procedure.

Figure. S4 shows an exploration of the effect of the noise level in Equation (6) of the main text on the GP prediction of the rate constant. Values of $\sigma_{noise}$ = 20, 30, and 50 were examined. The figure shows the predictions for these values as well as the TST rate constant (solid blue) and the fit to experiment (solid green). There is little difference between the results; we chose the 50 value because it was slightly better at low temperatures.

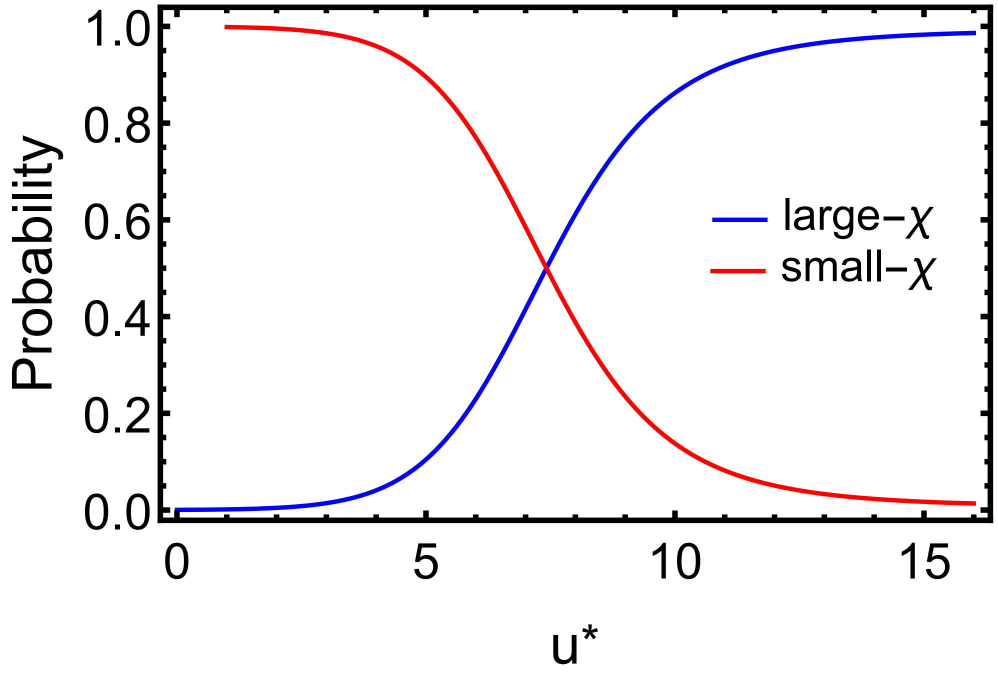


Figure S3: As a function of u*, the plot shows the probability of using the GP value for the large-$\chi$ cluster (blue) or the small-$\chi$ cluster (red).

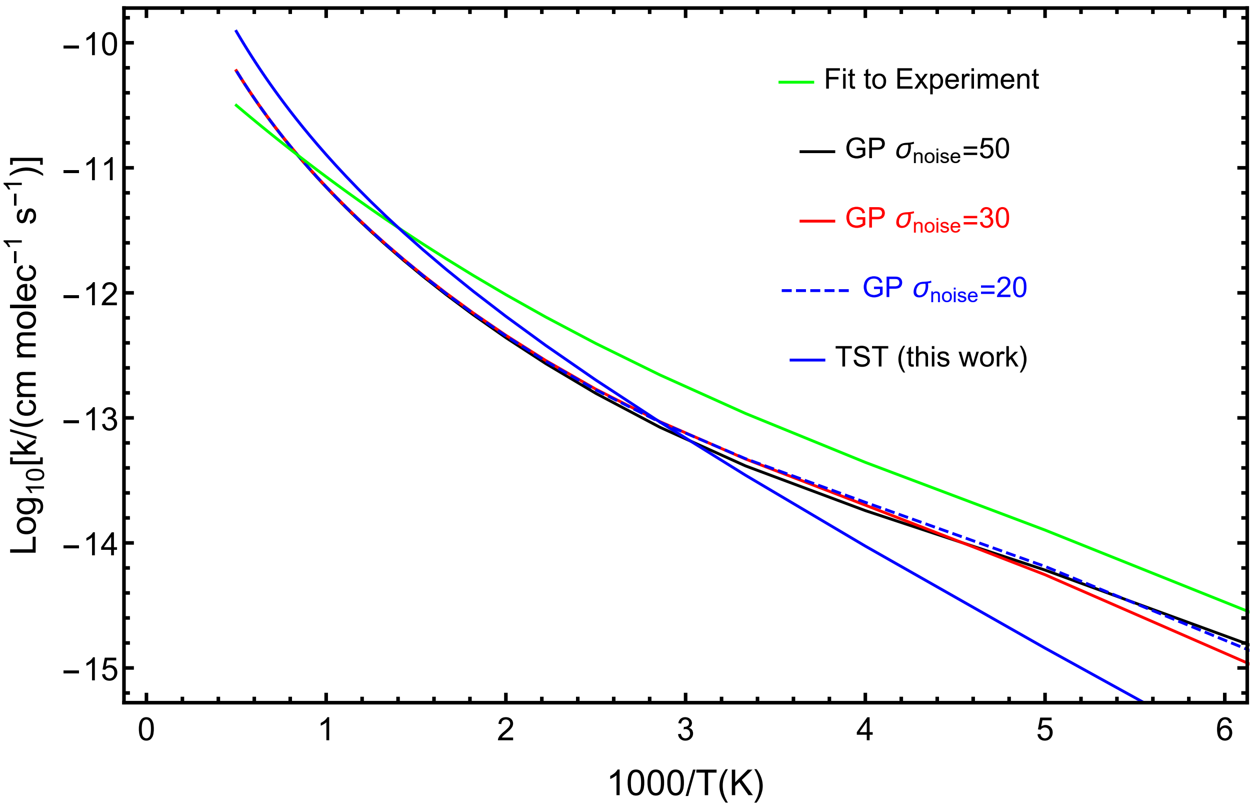


Figure S4: Gaussian Process predictions of the Cl + $CH_4$ rate constant for three different values, $\sigma_{noise}$, of the noise parameter in Equation (6) of the main text. The figure also shows the TST rate constants and the fit to the experimental rate constants.

# S-III. TST Rate Constant

Both Hoppe and Manthe (HM)[14] and Georgievskii and Klippenstein (GK)[15] have previously published calculations of the Transition State Theory (TST) rate constant as a function of temperature. The parameters for the barrier height to the forward reaction, the imaginary frequency of the barrier, and the barrier height for the reverse reaction are all similar. In neither case did the result of the TST calculation affect their final results, which were both in good agreement with experiment. Because our calculation starts from the TST result, and then corrects that result first with a simple Eckart correction and then with the Gaussian Process (GP) result, it is important for our method that we start with an accurate TST result. Unfortunately, the HM and GK TST results as published are not in good agreement with one another. We thus performed our own TST calculations, both treating the rotational partition function classically and evaluating it by direct count. Important references, particularly concerning the direct count, symmetry factors, and nuclear spin statistics, are those by McDowell[16,17] and Herzberg.[18] After correcting errors in our own calculation concerning nuclear spin degeneracies, and after identifying a zero-point energy error on their part, conversations with Hoppe and Manthe led us to agreement between their method and our methods, and fortunately all of them agreed with the result of GK. The result from our own calculation that we show in the figures in the main text, is nearly identical to that of GK.

# References


(1) Clyne, M. A. A.; Walker, R. F. Absolute Rate Constants for Elementary Reactions in the Chlorination of $CH_4$, $CD_4$, $CH_3Cl$, $CH_2Cl_2$, $CHCl_3$, $CDCl_3$ and $CBrCl_3$. *J. Chem. Soc., Faraday Trans. 1.* **1973**, *69*, 1547–1567.

(2) Manning, R. G.; Kurylo, M. J. Flash Photolysis Resonance Fluorescence Investigation of the Temperature Dependencies of the Reactions of Chlorine(2P) Atoms with Methane, Chloromethane, Fluoromethane, Excited Fluoromethane, and Ethane. *J. Phys. Chem.* **1977**, *81*, 291–296.

(3) Michael, J. V.; Lee, J. H. Selected Rate Constants for H, O, N, and Cl Atoms with Substrates at Room Temperatures. *Chem. Phys. Lett.* **1977**, *51*, 303–306.

(4) Whytock, D. A.; Lee, J. H.; Michael, J. V.; Payne, W. A.; Stief, L. J. Absolute Rate of the Reaction of Cl(2P) with Methane from 200–500 K. *J. Chem. Phys.* **1977**, *66*, 2690–2695.

(5) Keyser, L. F. Absolute Rate and Temperature Dependence of the Reaction between Chlorine (2P) Atoms and Methane. *J. Chem. Phys.* **1978**, *69*, 214–218.

(6) Zahniser, M. S.; Berquist, B. M.; Kaufman, F. Kinetics of the reaction $Cl + CH_4 \rightarrow CH_3 + HCl$ from 200° to 500° K. *Int. J. Chem. Kinet.* **1978**, *10*, 15–29.

(7) Ravishankara, A. R.; Wine, P. H. A Laser Flash Photolysis-Resonance Fluorescence Kinetics Study of the Reaction $Cl(2\,P) + CH_4 \rightarrow CH_3 + HCl$. *J. Chem. Phys.* **1980**, *72*, 25–30.

(8) Heneghan, S. P.; Knoot, P. A.; Benson, S. W. The Temperature Coefficient of the Rates in the System $Cl + CH_4 = CH_3 + HCl$, Thermochemistry of the Methyl Radical. *Int. J. Chem. Kinet.* **1981**, *13*, 677–691.

(9) Seeley, J. V.; Jayne, J. T.; Molina, M. J. Kinetic Studies of Chlorine Atom Reactions Using the Turbulent Flow Tube Technique. *J. Phys. Chem.* **1996**, *100*, 4019–4025.

(10) Pilgrim, J. S.; McIlroy, A.; Taatjes, C. A. Kinetics of Cl Atom Reactions with Methane, Ethane, and Propane from 292 to 800 K. *J. Chem. Phys. A.* **1997**, *101*, 1873–1880.

(11) Bryukov, M. G.; Slagle, I. R.; Knyazev, V. D. Kinetics of Reactions of Cl Atoms with Methane and Chlorinated Methanes. *J. Chem. Phys. A.* **2002**, *106*, 10532–10542.

(12) Allison, T. C.; Truhlar, D. G. In *Modern Methods for Multidimensional Dynamics Computations in Chemistry*; Thompson, D. L., Ed.; World Scientific: Singapore, 1998; pp 618–712.

(13) Nandi, A.; Bowman, J. M.; Houston, P. A Machine Learning Approach for Rate Constants. II. Clustering, Training, and Predictions for the O(3P) + HCl $\rightarrow$ OH + Cl Reaction. *J. Phys. Chem. A.* **2020**, *124*, 5746–5755.

(14) Hoppe, H.; Manthe, U. First-Principles Theory for the Reaction of Chlorine with Methane. *J. Phys. Chem. Lett.* **2022**, *13*, 2563–2566.

(15) Georgievskii, Y.; Klippenstein, S. J. Entanglement Effect and Angular Momentum Conservation in a Nonseparable Tunneling Treatment. *J. Chem. Theory Comput.* **2021**, *17*, 3863–3885.

(16) McDowell, R. S. Rotational Partition Functions for Spherical-top Molecules. *Journal of Quantitative Spectroscopy and Radiative Transfer* **1987**, *38*, 337–346.

(17) McDowell, R. S. Rotational Partition Functions for Symmetric-top Molecules. *J. Chem. Phys.* **1990**, *93*, 2801–2811.

(18) Herzberg, G. *Infrared and Raman Spectra of Polyatomic Molecules*; Molecular Spectra and Molecular Structure: II. Infrared; D. Van Nostrand: London, 1945; p 508ff.
